# Supplementary material for: Confinement of wave-function in Fractal geometry, a detection using DFT
Source: arXiv:1904.11862 source file (2019-11-19)
Supplement: Supplementary file 1 [file Supplimentary_info.pdf]

# Supplementary Information: Confinement of wave-function in Fractal geometry, a detection using DFT


Mohammed Ghadiyali* and Sajeev Chacko†

*Department of Physics, University of Mumbai,*
*Kalina Campus, Santacruz (E),*
*Mumbai - 400 098, India.*


## HEXAFLAKE

### Design of Hexaflake

The fractal hexaflake is constructed by first placing six CO molecule on a hexagon vertex and then a seventh in the centre on Cu(111) surface. As, the shape of the hexaflake closely relates to graphene, we have used the cell parameters and atomic position information of a molecular graphene [1]. A molecular graphene is an artificial lattice created on Cu(111) surface by placing CO molecules, such that formed lattice closely resembles to graphene. It is to be noted that we have only taken three atomic layers of Cu(111) and the structure optimization was only allowed in z-direction. This, methodology would not be accurate in most of the cases while studying surfaces, as during experimental realization there would be surface reconstruction due to thermal energy of the system. However, in the present case, the experimental realization would be done by the help of scanning tunnelling microscope (STM) at very low temperatures, which would arrest the motion of the atoms. This methodology have been used by Paavilainen *et. al.* [2] for modelling of kagome lattice made up of CO molecules on Cu(111) and for experimental realization the work of Manoharan *et. al.* [1] can be referred.

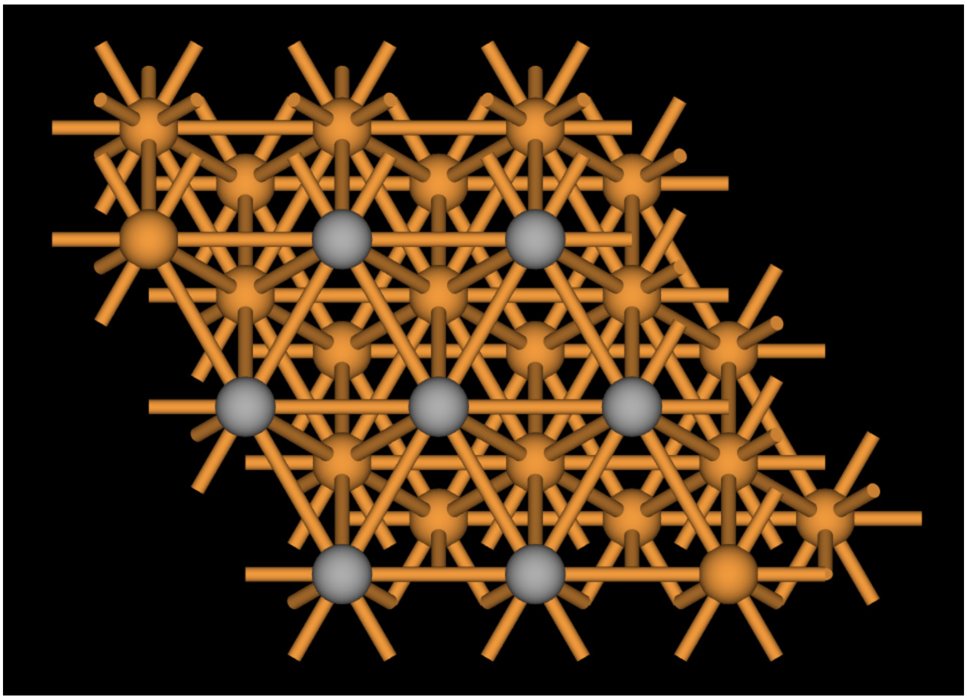

FIG. 1: (colour online) The image above represents the image of artificial lattice in the form of fractal hexaflake, it is on a Cu(111) surface by selective placing CO molecules.

**Application of electrical Field**

For study the effect of the application of electric field on Hexaflake, we have applied an electrical filed in the z-direction (perpendicular to the plane of the page, w.r.t figure 1) on the system. The field strengths were 0.2, 0.4 and 0.6 volts/nm and they are marked as b, c and d, respectively in the figure 2. It is obvious, that there is no change in the Fractal dimension of hexaflake on application of electrical field, demonstrating the stable nature of its Hausdorff dimension. An in depth study would be required to understand the underling reasons for this behaviour. However, it can be

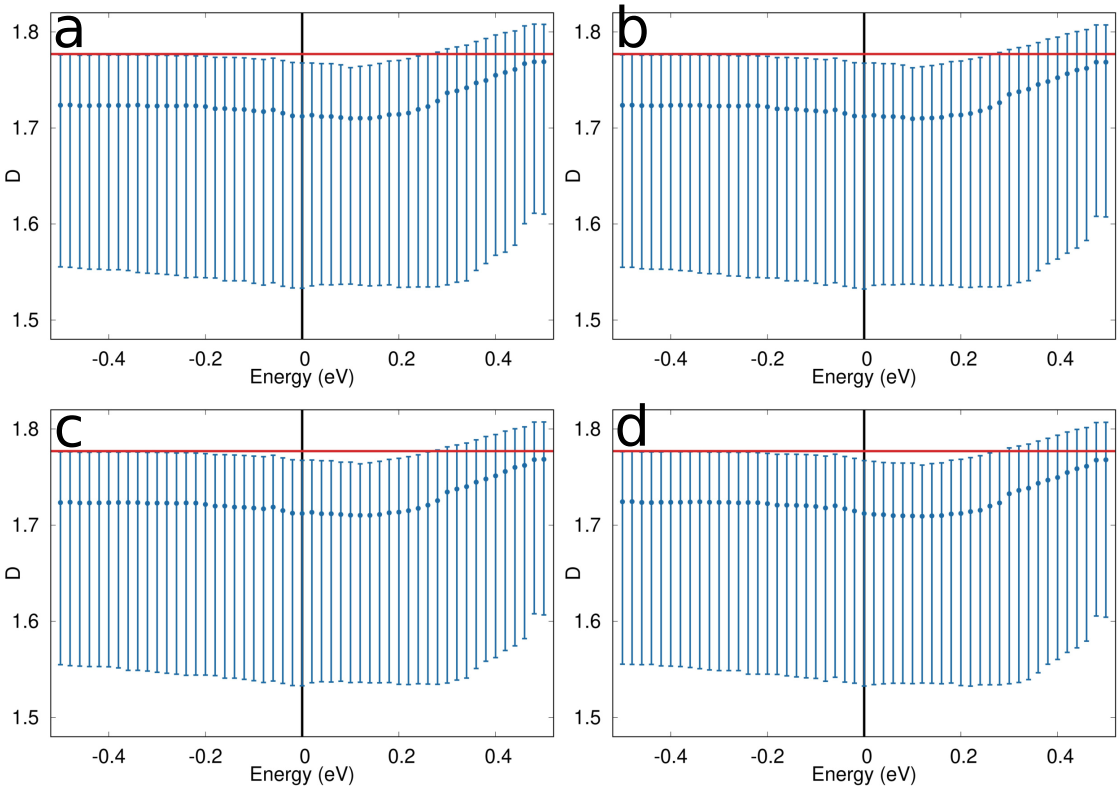


FIG. 2: (colour online) The fractal dimensions under the influence of electrical file of strength of 0.0, 0.2, 0.4 and 0.6 volts/nm is given in sub-figure a, b c and d, respectively. Here the copper atoms are represented by the brownish-orange colour, while the red colour represents the oxygen of CO molecule.

## VICSEK FRACTAL

### Design of Vicsek Fractal

The Vicsek Fractal is formed by repeating pattern of crosses such that a snow flake type structure can be formed. To model this we have taken an inspiration form artificial Lieb lattice, which is created by placing CO molecules on Cu(111) surface [3]. Again, lattice parameters and atomic positions for CO molecules is taken from the experimental work cited above and then placed on a Cu(111) surface. It is to be noted that the Lieb lattice can also be created with other atomic structures, such as Cl vacancy on chlorinated Cu(100) [4]. However, due size constrains in DFT we have selected current system. Again, we have taken three atom layer thick Cu surface and optimization is performed in z-direction only.

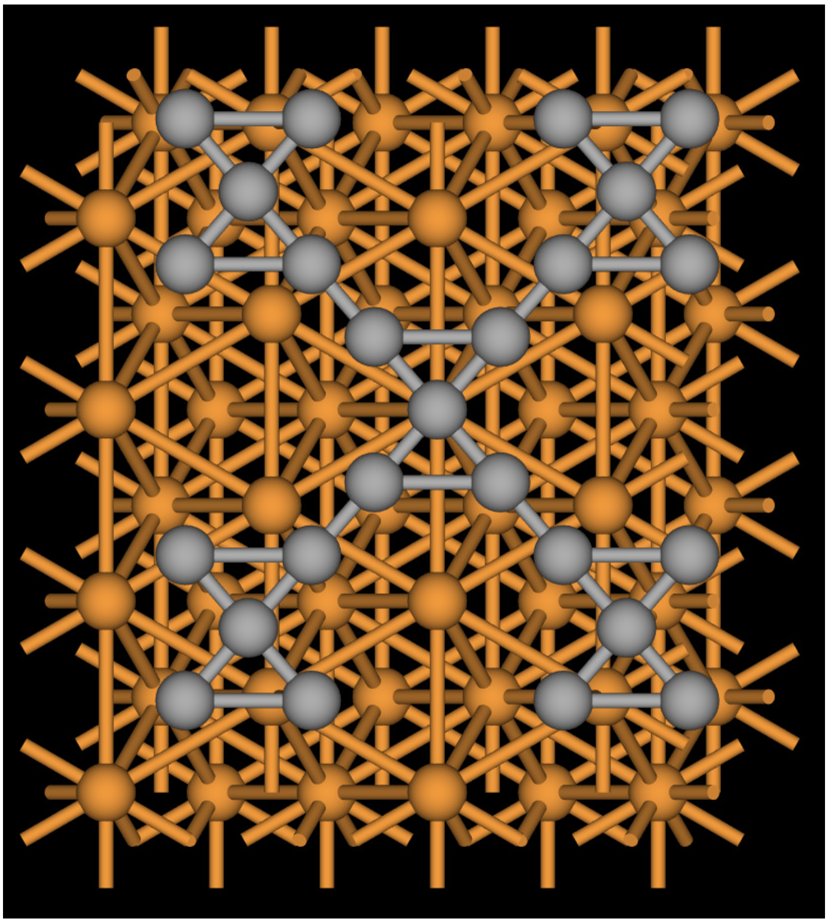

FIG. 3: (colour online) The image above represents a snow flake version of Vicsek Fractal created by CO molecules on Cu(111) surface. The colour scheme is same as above (Hexaflake)

## BENZENE ON CU(111)

For this system, a benzene molecule is placed on Cu(111) surface at a random position at a hight of ≈2 Å with the lowermost layer set to be fixed. Then the system was allowed to relaxed without any constrains. The final optimized geometry is provide in figure 4.

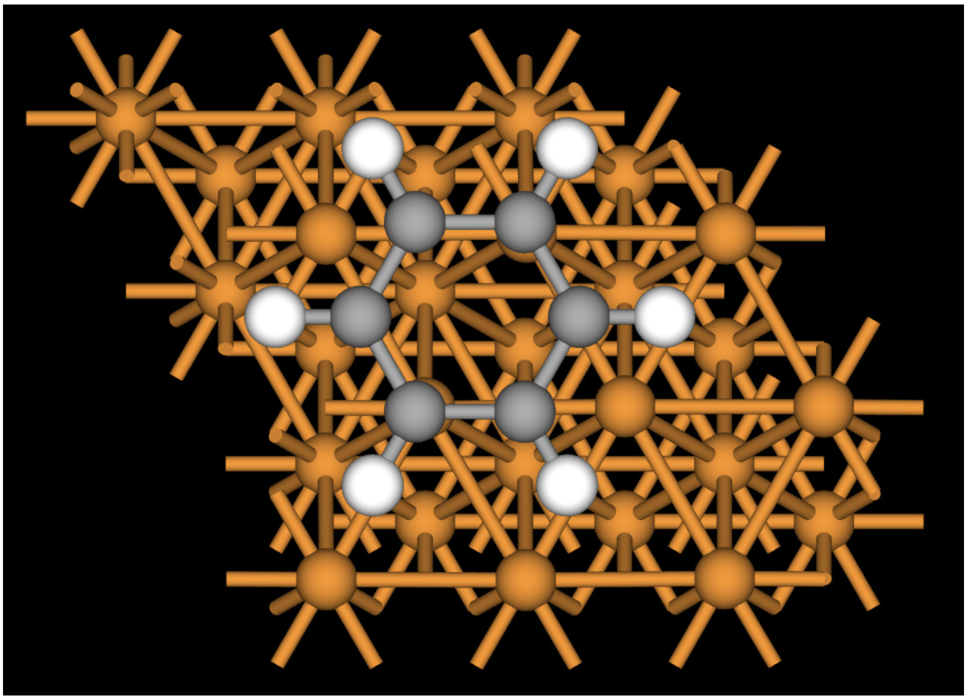

FIG. 4: (colour online) Benzene on Cu(111) surface. Note this is one of the possible configuration by which benzene can be adsorb on Cu surface, we have randomly selected one, as to demonstrated that only image analysis methodology is not sufficient for demonstrating wavefunction confinement in Fractal dimensions.

* Electronic address: ghadiyali.mohd@physics.mu.ac.in
† Electronic address: sajeev.chacko@physics.mu.ac.in; sajeev.chacko@gmail.com

[1] Warren Mar Wonhee Ko Francisco Guinea Gomes, Kenjiro K. and Hari C. Manoharan. Designer dirac fermions and topological phases in molecular graphene. *Nature*, 483(7389):306, 2012.
[2] Sami Paavilainen, Matti Ropo, Jouko Nieminen, Jaakko Akola, and Esa Rasanen. Coexisting honeycomb and kagome characteristics in the electronic band structure of molecular graphene. *Nano letters*, 16(6):3519–3523, 2016.
[3] Thomas S. Gardenier Peter H. Jacobse Guido CP van Miert Sander N. Kempkes Stephan JM Zevenhuizen Cristiane Morais Smith Daniel Vanmaekelbergh Slot, Marlou R. and Ingmar Swart. Experimental realization and characterization of an electronic lieb lattice. *Nature Physics*, 12(7):672, 2017.
[4] FE Kalff, Marnix P Rebergen, E Fahrenfort, Jan Girovsky, Ranko Toskovic, Jose L Lado, Joaquín Fernández-Rossier, and Alexander F Otte. A kilobyte rewritable atomic memory. *Nature nanotechnology*, 11(11):926, 2016.
